# Supplementary material for: LearnedFTL: A Learning-Based Page-Level FTL for Reducing Double Reads in Flash-Based SSDs
Source: arXiv:2303.13226 source file (2024-04-25)
Supplement: Supplementary file 1 [file Appendix.tex]

% \appendix
%   \renewcommand{\appendixname}{Appendix~\Alph{section}
% %   FGHSAEHSHH
%   }
%   \section{Key Modifications}
